# Supplementary material for: A Tighter Complexity Analysis of SparseGPT
Source: arXiv:2408.12151 source file (2024-10-18)
Supplement: Supplementary file 1 [file 6_appendix.tex]

\section{Limitations}\label{sec:limit}
% This work has not directly addressed the practical applications of our results, as we have not
% implemented our tensor attention algorithm. Future research could investigate how these findings
% could be applied in real-world scenarios.

This work has not directly addressed the practical applications, as we have not designed or implemented any algorithm. We focus on the theoretical analysis of the time complexity of SparseGPT. Future research could investigate how these findings could be used to design more efficient algorithms and applied in real-world scenarios.

\section{Societal Impacts}\label{sec:impact}

% We delve into and offer a deeper understanding of the attention mechanism, introducing a novel
% approach to integrate multi-modality into attention through the tensor attention algorithm. We
% also demonstrate that the computation of both forward and backward tensor attention can be
% achieved with almost linear time complexity.
% Regarding the negative societal impact, since our work is completely theoretical in nature, we
% do not foresee any potential negative societal impacts which worth pointing out.

We delve into and offer a deeper understanding of the time complexity of SparseGPT by incoporating the techniques from fast matrix multiplication and analyzing lazy update strategies in iterative maintenance problems. Regarding the negative societal impact, since our work is completely theoretical in nature, we do not foresee any potential negative societal impacts which worth pointing out.
